# Supplementary material for: Motorway Traffic Flow Prediction using Advanced Deep Learning
Source: arXiv:1907.06356 source file (2019-07-17)
Supplement: Supplementary file 1 [file appendix_fig_runtime.tex]

%!TEX root = ../IEEE_ITSC_2019.tex
%
